# Supplementary material for: Benchmarking Generative Models on Computational Thinking Tests in Elementary Visual Programming
Source: arXiv:2406.09891 source file (2025-03-18)
Supplement: Supplementary file 1 [file 9.6_appendix_datasheet.tex]

\clearpage
\section{Datasheet}
\label{app-sec.datasheet}

We include the datasheet \cite{DBLP:journals/cacm/GebruMVVWDC21} for both our curated benchmark and the synthetically generated dataset. 

\subsection{Motivation}
\textbf{For what purpose was the dataset created?}

The benchmark was curated for assessing generative models' computational thinking and problem-solving skills on tasks designed for school students. It is comprised of three parts, namely \hocType{}, \aceType{} and \ctType{}. \hocType{} is used to analyze the models' solution synthesis capabilities under strict constraints, while \aceType{} and \ctType{} are made for assessing the models' problem-solving skills over three cognitive levels: \Analyzing{}, \Evaluating{}, and \Creating{}.

\looseness-1The synthetic dataset was generated to improve the models' performance on computational thinking and problem-solving tasks (e.g., via fine-tuning). We aim to accomplish two objectives with the dataset: improve performance on tasks assessed by the benchmark (i.e., solution synthesis and multi-choice questions) and offer the models a better understanding of visual programming via training on fine-grained skills.

\textbf{Who created the dataset (e.g., which team, research group) and on behalf of which entity (e.g., company, institution, organization)?}

The benchmark was curated by the authors of the original paper from sources such as  \cite{DBLP:conf/sigcse/GhoshMS24,DBLP:journals/chb/Roman-GonzalezP17,hourofcode_maze}, while the synthetic dataset was created by the authors, using techniques from literature \cite{padurean2024neural,DBLP:conf/iclr/BunelHDSK18,DBLP:conf/nips/AhmedCEFGRS20}. Full details regarding the authors of the original paper will be given at the time of publication.

\textbf{Who funded the creation of the dataset?}

Full details regarding funding will be given at the time of publication.

\textbf{Any other comments?}

None.

\subsection{Composition}

\textbf{What do the instances that comprise the dataset represent (e.g., documents, photos, people, countries)?}

The dataset comprises grid representations, codes (under AST structure or in Python), traces (i.e., sequences of grids), sequences of basic actions, instructions, and answer options for multi-choice questions and explanations involving reasoning about the answers. The tasks in the benchmark also contain images which are visual representations of the grids in the dataset. We also include prompt templates for easily generating prompts.

For ease of usage, we offer a method for accessing data in a uniform way. In this data representation, all records have a task type (i.e., what kind of task they represent -- see \iftoggle{MainSuppContent}{Section~\ref{sec.dataset}}{Section~4}), an instruction (i.e., for multi-choice questions), a set of grids, a set of codes, answer options (i.e., for multi-choice questions), and an answer. Additionally, they contain a miscellaneous field that includes any information necessary for the respective tasks (e.g., traces, explanations).

\textbf{How many instances are there in total (of each type, if appropriate)?}

There are $111,861$ synthetic data points for training, $2,538$ synthetic data points for evaluating, and $65$ tasks in the real-world benchmark.

\textbf{Does the dataset contain all possible instances or is it a sample (not
necessarily random) of instances from a larger set?}

Only in the case of \ctType{}, the data is a sample of 24 tasks out of a total of 28 tasks, due to incompatibility reasons.

\textbf{What data does each instance consist of? }

Each instance consists of the grid representation, its solution code, usually a type of task and an answer and additional data for formulating the question, answer, or explanations (e.g., trace of grid state or sequence of basic actions).

\textbf{Is there a label or target associated with each instance?}

Yes, possible target answers are included.

\textbf{Is any information missing from individual instances?}

Not to our knowledge.

For the uniform access method, some fields are empty due to the nature of the task.

\textbf{Are relationships between individual instances made explicit (e.g.,
users’ movie ratings, social network links)?}

No.

\textbf{Are there recommended data splits (e.g., training, development/validation, testing)?} 

Yes, the data is naturally split into real-world evaluation (i.e., benchmark), synthetic evaluation (i.e., synthetic data), and training (i.e., synthetic data) segments. The training data is further randomly split into train (i.e., 90\% of synthetic data) and validation (i.e., 10\% of synthetic data).

\textbf{Are there any errors, sources of noise, or redundancies in the dataset?}

The benchmark is created by experts and does not have errors to the best of our knowledge. The synthetic dataset was verified automatically while being created. However, it has not been manually checked for errors or redundancies that may get past automatic checks.

\textbf{Is the dataset self-contained, or does it link to or otherwise rely on
external resources (e.g., websites, tweets, other datasets)?}

The dataset is self-contained.

\textbf{Does the dataset contain data that might be considered confidential (e.g., data that is protected by legal privilege or by doctor–patient confidentiality, data that includes the content of individuals’ non-public communications)?}

No.

\textbf{Does the dataset contain data that, if viewed directly, might be offensive, insulting, threatening, or might otherwise cause anxiety?}

No.

\textbf{Does the dataset identify any subpopulations (e.g., by age, gender)?}

No.

\textbf{Is it possible to identify individuals (i.e., one or more natural persons), either directly or indirectly (i.e., in combination with other data) from the dataset?}

No.

\textbf{Does the dataset contain data that might be considered sensitive in
any way (e.g., data that reveals race or ethnic origins, sexual orientations, religious beliefs, political opinions or union memberships, or locations; financial or health data; biometric or genetic data; forms of government identification, such as social security numbers; criminal history)?}

No.

\textbf{Any other comments?}

None.

\subsection{Collection Process}

\textbf{How was the data associated with each instance acquired?}

The data used for benchmarking was collected from each respective source \cite{DBLP:conf/sigcse/GhoshMS24,DBLP:journals/chb/Roman-GonzalezP17,hourofcode_maze} and translated to our representation. The synthetic dataset was created by the authors, using techniques from literature \cite{padurean2024neural,DBLP:conf/iclr/BunelHDSK18,DBLP:conf/nips/AhmedCEFGRS20}.

\textbf{What mechanisms or procedures were used to collect the data (e.g., hardware apparatuses or sensors, manual human curation, software programs, software APIs?}

The data used for benchmarking was collected via manual curation, while the synthetic dataset was produced by authors' own software using techniques from literature \cite{padurean2024neural,DBLP:conf/iclr/BunelHDSK18,DBLP:conf/nips/AhmedCEFGRS20}.

\textbf{If the dataset is a sample from a larger set, what was the sampling strategy (e.g., deterministic, probabilistic with specific sampling probabilities)?}

While curating data from \ctType{}, we kept the data compatible with our representation of a grid.

\textbf{Who was involved in the data collection process (e.g., students, crowdworkers, contractors) and how were they compensated (e.g., how much were crowdworkers paid)?}

The authors were the only involved in the data collection process.

\textbf{Over what timeframe was the data collected?}

The data was collected between February and May 2024. It is not known to the authors when the \hocType{} lesson~\cite{hourofcode_maze} was created. Data for \aceType{} was published in 2024, while data for \ctType{} was published in 2017.

\textbf{Were any ethical review processes conducted (e.g., by an institutional review board)?}

No.

\textbf{Did you collect the data from the individuals in question directly, or obtain it via third parties or other sources (e.g., websites)?}

N/A.

\textbf{Were the individuals in question notified about the data collection?}

N/A.

\textbf{Did the individuals in question consent to the collection and use of
their data?}

N/A.

\textbf{If consent was obtained, were the consenting individuals provided
with a mechanism to revoke their consent in the future or for certain
uses?}

N/A.

\textbf{Has an analysis of the potential impact of the dataset and its use
on data subjects (e.g., a data protection impact analysis) been con-
ducted?}

N/A.

\textbf{Any other comments?}

None.

\subsection{Preprocessing/cleaning/labeling}

\textbf{Was any preprocessing/cleaning/labeling of the data done (e.g., discretization or bucketing, tokenization, part-of-speech tagging, SIFT
feature extraction, removal of instances, processing of missing values)?}

No.

\textbf{Was the ``raw'' data saved in addition to the preprocessed/cleaned/labeled data (e.g., to support unanticipated future uses)?}

N/A.

\textbf{Is the software that was used to preprocess/clean/label the data available?}

N/A.

\textbf{Any other comments?}

None.

\subsection{Uses}

\textbf{Has the dataset been used for any tasks already?}

The curated data was previously used in their intended ways by the authors of each of \cite{DBLP:conf/sigcse/GhoshMS24,DBLP:journals/chb/Roman-GonzalezP17,hourofcode_maze}. The synthetic dataset was only used in the original paper.

\textbf{Is there a repository that links to any or all papers or systems that use the dataset?}

There will be a publicly released repository at the time of publication.

\textbf{What (other) tasks could the dataset be used for?}

The dataset can be used for any purpose requiring various computational thinking tasks, or the grids and codes involved. The original paper uses them for fine-tuning large language models, but researchers are free to use them in other ways to improve generative models' performance and not only.

\textbf{Is there anything about the composition of the dataset or the way it
was collected and preprocessed/cleaned/labeled that might impact future uses?}

No.

\textbf{Are there tasks for which the dataset should not be used?}

Training on this data does not guarantee generalization to other domains.

\textbf{Any other comments?}

None.

\subsection{Distribution}

\textbf{Will the dataset be distributed to third parties outside of the entity (e.g., company, institution, organization) on behalf of which the
dataset was created?}

Yes, it will be free and available online at the time of publication.

\textbf{How will the dataset will be distributed (e.g., tarball on website, API,
GitHub)?}

The dataset will be available on GitHub at the time of the oringial paper's publication, under CC BY-NC-SA 4.0 license. The source code for processing data and evaluating models will be available under MIT license.

\textbf{When will the dataset be distributed?}

The dataset will be distributed at the time of the original paper's publication.

\textbf{Will the dataset be distributed under a copyright or other intellectual property (IP) license, and/or under applicable terms of use (ToU)?}

The data will be distributed under CC BY-NC-SA 4.0 license.

\textbf{Have any third parties imposed IP-based or other restrictions on the data associated with the instances?}

No.

\textbf{Do any export controls or other regulatory restrictions apply to the dataset or to individual instances?}

No.

\textbf{Any other comments?}

None.

\subsection{Maintenance}

\textbf{Who will be supporting/hosting/maintaining the dataset?}

The authors of the paper will provide needed maintenance to the dataset. Further work may add additional domains to the data and contributors are free to submit pull requests.

\textbf{How can the owner/curator/manager of the dataset be contacted
(e.g., email address)?}

The authors will make this data public at the time of the original paper's publication.

\textbf{Is there an erratum?}

No.

\textbf{Will the dataset be updated (e.g., to correct labeling errors, add
new instances, delete instances)?}

Further work may choose to add more data (e.g., more tests, or synthetic data for Karel).

\textbf{If the dataset relates to people, are there applicable limits on the retention of the data associated with the instances (e.g., were the individuals in question told that their data would be retained for a fixed
period of time and then deleted)?}

N/A.

\textbf{Will older versions of the dataset continue to be supported/hosted/maintained?}

In case new data will be released, a versioning system will be used to keep track of versions.

\textbf{If others want to extend/augment/build on/contribute to the dataset,
is there a mechanism for them to do so?}

We plan to use GitHub for maintaining both the code and the data. Contributors can either contact authors or submit pull requests.

\textbf{Any other comments?}

None.
