# Supplementary material for: Benchmarking Generative Models on Computational Thinking Tests in Elementary Visual Programming
Source: arXiv:2406.09891 source file (2025-03-18)
Supplement: Supplementary file 2 [file fig_techniques.tex]

% !TEX root =  main.tex
%%%%%%%%%%%%%%%%%%%%%%%%%%%%%%%%%%%
%%%%%%%%%%%%%%%%%%%%%%%%%%%%%%%%%%%
\begin{figure*}[h!]
\centering
    \scalebox{0.75}{
        \setlength\tabcolsep{2pt}
        \aboverulesep=0pt
        \belowrulesep=0pt
        
        \begin{tabular}{llllll}  
            \toprule
             \multirow[c]{2}{*}[0mm]{{\backslashbox[50mm]{\textbf{Technique}}{\textbf{Attributes}}}} &
             \multicolumn{1}{c}{\textbf{Base model}} &
             \multicolumn{2}{c}{\textbf{Grid representation}} &
             \multicolumn{1}{c}{\textbf{Fine-tuned on}} &
             \multicolumn{1}{c}{\textbf{Explanation}} \\

            \cmidrule(lr){3-4}
            
             & 
             &
             \multicolumn{1}{c}{\textbf{Visual}} &
             \multicolumn{1}{c}{\textbf{Text}} &
             &
             \\
            
            \midrule
            $\TechLlamaSeven$ &
            CodeLlama \cite{DBLP:journals/corr/abs-2308-12950} &
            No &
            Yes &
            N/A &
            N/A \\

            $\TechLlava$ &
            LLaVA v1.5 \cite{DBLP:conf/nips/LiuLWL23a} &
            Yes &
            Yes &
            N/A &
            N/A \\

            \rowcolor{red!15}
            $\TechLlamaThreeEight$ &
            Llama3 \cite{Llama3} &
            No &
            Yes &
            N/A &
            N/A \\

            \midrule
            $\TechChatGPT$ &
            GPT-3.5 \cite{ChatGPT} &
            No &
            Yes &
            N/A &
            N/A \\

            $\TechGPTFourV$ &
            GPT-4V \cite{GPT4V} &
            Yes &
            No &
            N/A &
            N/A \\

            $\TechGPTFour$ &
            GPT-4 \cite{GPT4} &
            No &
            Yes &
            N/A &
            N/A \\

            $\TechGPTFourVCombined$ &
            GPT-4V \cite{GPT4V} &
            Yes &
            Yes &
            N/A &
            N/A \\

            $\TechGPTFourOVision$ &
            GPT-4o \cite{GPT4o} &
            Yes &
            No &
            N/A &
            N/A \\

            $\TechGPTFourO$ &
            GPT-4o \cite{GPT4o} &
            No &
            Yes &
            N/A &
            N/A \\

            \rowcolor{orange!15}
            $\TechGPTFourOCombined$ &
            GPT-4o \cite{GPT4o} &
            Yes &
            Yes &
            N/A &
            N/A \\

            \midrule
            $\TechHocFinetuneNoExpThree$&
            Llama3 \cite{Llama3} &
            No &
            Yes &
            Solution synthesis &
            None \\

            $\TechPlainFinetuneThree$&
            Llama3 \cite{Llama3} &
            No &
            Yes &
            Solution synthesis + MCQ&
            None \\

            $\TechHocFinetuneExpThree$&
            Llama3 \cite{Llama3} &
            No &
            Yes &
            Solution synthesis &
            At training \\

            $\TechTopFinetuneThree$&
            Llama3 \cite{Llama3} &
            No &
            Yes &
            Solution synthesis + MCQ&
            At training \\

            \rowcolor{green!60!black!15}
            $\TechHierFinetuneThree$&
            Llama3 \cite{Llama3} &
            No &
            Yes &
            Full data &
            At training \\

            $\TechHierEmuFinetuneEmuInfThree$&
            Llama3 \cite{Llama3} &
            No &
            Yes &
            Full data &
            At training and inference \\

            \bottomrule   
        \end{tabular}
        }
    \vspace{-1mm}
    \caption{Table showing the techniques based on generative models. We mention the base generative model and whether we represent the grid visually or in text. For the fine-tuned models (i.e., \TechLlamaCT{}), we mention the data segment it was trained on and whether it was trained with no explanations, to produce an explanation, or to receive a correct explanation at inference time.}
    \label{fig.experiments.techniques}
    \vspace{-6mm}
    %%%%%%%%%%%%%%%%%
\end{figure*}
